# Supplementary material for: Reducing Electricity Demand Charge for Data Centers with Partial Execution
Source: arXiv:1307.5442 source file (2013-12-17)
Supplement: Supplementary file 1 [file appendix.tex]

\appendices

\section{Proof of Lemma~\ref{lem:beta}}
\label{proof:beta}

The KKT conditions \cite{BV04} of the per-stub datacenter problem \eqref{opt:per-stubdc} constitute the following system of equations.
\begin{align}
	\hspace{-2mm}\rho(\beta^{t+1}_{ij}-\alpha^{t+1}_{ij}) + D_i(P^B_j+ \nu^{t+1}_{j}) - \lambda^t_{ij} -\tau^{t+1}_{ij} &= 0,\forall i,\label{kkt:per-stubdc:optimality} \\
			  \nu^{t+1}_j\Big(C_j - \sum_i \beta^{t+1}_{ij}D_i\Big) = 0, \beta^{t+1}_{ij}\tau^{t+1}_{ij} & = 0,\forall i \label{kkt:per-stubdc:slackness} \\
	C_j - \sum_i \beta^{t+1}_{ij}D_i \ge 0,\nu_j \ge 0, \beta^{t+1}_{ij} \ge 0,\tau^{t+1}_{ij} & \ge 0, \forall i. \label{kkt:per-stubdc:primal}
\end{align}
$\beta^{t+1}_{ij}$ is the optimal solution, and $\nu^{t+1}_j$ is the KKT multiplier. \eqref{kkt:per-stubdc:optimality} is the first-order optimality conditions, \eqref{kkt:per-stubdc:slackness} is the complementary slackness condition, and \eqref{kkt:per-stubdc:primal} are the primal and dual feasibility conditions.

For all $i\in\mathcal{I}$ that satisfy $\lambda^t_{ij}-D_i P^B_j+\rho\alpha^{t+1}_{ij} \le 0$, assume $\beta^{t+1}_{ij}>0$. Then according to the complementary slackness condition \eqref{kkt:per-stubdc:slackness} $\tau^{t+1}_{ij}=0$. The left hand side (LHS) of \eqref{kkt:per-stubdc:optimality} is always positive, which contradicts the optimality condition. Thus $\beta^{t+1}_{ij}=0$.

As in Lemma~\ref{lem:beta}, denote the rest of stub datacenters as the set $\mathcal{I}^{t+1}_j$. $\lambda^t_{ij}-D_i P^B_j+\rho\alpha^{t+1}_{ij} > 0$ holds for all $i\in\mathcal{I}_j^{t+1}$. If $\sum_{i\in\mathcal{I}^{t+1}_j} (\lambda^t_{ij}-D_i P^B_j+\rho\alpha^{t+1}_{ij})D_i \le \rho C_j$, then according to \eqref{kkt:per-stubdc:slackness} $\nu^{t+1}_j=0$. This is so because for those $i\in\mathcal{I}^{t+1}_j$ such that $\beta^{t+1}_{ij}>0$, $\rho\beta^{t+1}_{ij}\le \lambda^t_{ij}-D_i P^B_j+\rho\alpha^{t+1}_{ij}$ since $\nu^{t+1}_j\ge 0$ in \eqref{kkt:per-stubdc:optimality}. Thus $\sum_{i\in\mathcal{I}^{t+1}_j}\beta^{t+1}_{ij}D_i \le C_j$, and $\nu^{t+1}_j= 0$. Then, $\tau^{t+1}_{ij}=0$ must hold for all $i\in\mathcal{I}_j^{t+1}$, for otherwise $\beta^{t+1}_{ij}=0$ and the LHS of \eqref{kkt:per-stubdc:slackness} is always negative. Substituting $\nu^{t+1}_j=0$ and $\tau^{t+1}_{ij}=0$ into \eqref{kkt:per-stubdc:optimality} yields $\beta^{t+1}_{ij} = \frac{\lambda^t_{ij}-D_i P^B_j}{\rho}+\alpha^{t+1}_{ij}$.

If $\sum_{i\in\mathcal{I}^{t+1}_j} (\lambda^t_{ij}-D_i P^B_j+\rho\alpha^{t+1}_{ij})D_i > \rho C_j$, note that the objective of \eqref{opt:per-stubdc} is minimized at $\frac{\lambda^t_{ij}-D_i (P^B_j+\nu^{t+1}_j )}{\rho}+\alpha^{t+1}_{ij}>0$ when the capacity constraint is absent, we must have $\beta^{t+1}_{ij}<\frac{\lambda^t_{ij}-D_i (P^B_j+\nu^{t+1}_j)}{\rho}+\alpha^{t+1}_{ij}$ to conform to the capacity constraint. Since the objective function of \eqref{opt:per-stubdc} is convex in $\beta_{ij}$, for $\beta_{ij}\in\Big[0,\frac{\lambda^t_{ij}-D_i (P^B_j+\nu^{t+1}_j)}{\rho}+\alpha^{t+1}_{ij}\Big]$ it is increasing. Thus the optimal $\beta_{ij}^{t+1}$ must satisfy the capacity constraint at equality, and equal to $\max\left\{\frac{\lambda^t_{ij}-D_i (P^B_j+\nu^{t+1}_j)}{\rho}+\alpha^{t+1}_{ij},0\right\}$.

\section{Proof of Lemma~\ref{lem:alpha}}
\label{proof:alpha}

The KKT conditions for the per-client sub-problem with an affine utility function \eqref{opt:per-client-affine} are
\begin{align}
	\hspace{-5mm}\rho(\alpha^{t+1}_{ij}-\beta^t_{ij}) + D_i(a L_{ij}+ P^E_j) + \lambda^t_{ij}\nonumber\\ 
	+ \mu^{t+1}_{i} -\sigma^{t+1}_{ij} &= 0,\forall j,\label{kkt:per-client:optimality} \\
				  \sum_j \alpha^{t+1}_{ij} -1&=0,\label{kkt:per-client:primal}	  \\
	\mu_i^{t+1}\ne 0, \sigma^{t+1}_{ij}\alpha^{t+1}_{ij}  =0,\alpha^{t+1}_{ij} \ge 0, \sigma^{t+1}_{ij} & \ge 0,\forall j, \label{kkt:per-client:dual}
\end{align}
where $\alpha^{t+1}_{ij}$ is the optimal solution as in \eqref{eqn:x-min}, and $\mu_i^{t+1}$ and $\sigma^{t+1}_{ij}$ are the KKT multiplier for the equality and inequality constraints of \eqref{opt:per-client-affine}, respectively. \eqref{kkt:per-client:optimality} corresponds to the first-order optimality condition, \eqref{kkt:per-client:primal} is one of the primal feasibility conditions, and \eqref{kkt:per-client:dual} captures the other primal feasibility condition, the dual feasibility, and the complementary slackness conditions. Essentially, since $\alpha^{t+1}_{ij}$ and $\sigma^{t+1}_{ij}$ never appear at the same time in \eqref{kkt:per-client:optimality}, $\alpha^{t+1}_{ij}=\max\left\{\beta^{t}_{ij}-\left(D_i\left(a L_{ij}+P^E_j\right) + \lambda^t_{ij}+\mu_i^{t+1}\right)/{\rho},0\right\}$, and must satisfy \eqref{kkt:per-client:primal}. Thus the proof.
